# Supplementary material for: "Don't Step on My Toes": Resolving Editing Conflicts in Real-Time Collaboration in Computational Notebooks
Source: arXiv:2404.04695 source file (2024-04-06)
Supplement: Supplementary file 1 [file 05.5_additional_evaluation.tex]

\section{Planning Session: Planning for Various Collaboration Scenarios}
\add{Noticeably, none of the participants used the cell-level access control and variable-level access control features when working with the clumsy collaborator in the paired session, although they have mentioned the potential of using these features in other collaboration setups.
To better understand the usefulness of \sys{} under various collaboration scenarios, we conducted an additional evaluation where we asked participants to plan a future collaboration session by configuring a collaborative notebook.
This additional evaluation allowed us to explore the usefulness of the \sys{} features in different collaboration scenarios. 
By asking participants to configure a collaborative notebook for planning a future collaboration session, we were able to see how they would use the collaborative features in a more proactive manner. 
This can provide valuable insights into how users might use the features of \sys{} in a variety of collaborative environments.}

\add{Overall, our additional evaluation showed that the \sys{} features can be useful in various collaboration scenarios, including working on an asynchronous paired programming session, working on tasks with high cost of error recovery, and using collaborative notebooks as lecture notes. 
By providing a way to prevent conflicts and improve organization, \sys{} can help make collaboration more efficient and effective.}
\add{\subsection{Study Setup}}
\add{In the individual study sessions, we used the same deployment as in the paired sessions. 
Based on participants' responses from the previous study, where they mentioned their prior or future use of collaborative notebooks, we synthesized three collaboration scenarios designed to be representative of various realistic situations.
For each scenario, we gave participants an initial notebook containing skeleton code and a written description of the collaboration scenario.
We asked participants to plan for the collaboration by leveraging the features of \sys{} and modifying the notebook content as necessary. 
When they finished planning, we asked participants to verbally describe their plans to the study coordinators, who would then ask a set of semi-structured interview questions to gain further insight into the participants' plans and the features they used or did not use, as well as any potential problems that might arise during the collaboration and any additional features that they felt would be useful. 
Participants were given as much time as they needed to think about their plans, with most individual sessions lasting around 30 minutes.}
\add{\subsection{Collaboration Scenarios}}
\add{In the individual session, participants were asked to plan for the following three collaboration scenarios:}
\subsubsection{Scenario 1: Asynchronous Collaboration with a Peer}
\add{For the first scenario, participants are asked to plan a paired programming session with a friend named Bob who is inexperienced with libraries like Pandas and Numpy, similar to the clumsy collaborator case in the previous study. 
However, due to conflicting schedules, Bob and the participant are unable to find a synchronous time to work together. 
This means that both of them may join and leave the session with incomplete code, and the participant cannot guarantee how Bob will use the collaborative editing features without being able to observe and intervene in Bob's actions.}
\subsubsection{Scenario 2: Working with Trainees and a High Cost of Error Recovery} 
\add{
In this scenario, we asked participants to plan a collaboration session as a full-time employee distributing tasks to interns on visualizing different aspects of the data. 
We provided participants with a notebook skeleton where the data takes a long time to load. 
In this scenario, participants needed to avoid the shared dataframe being polluted by any accidental changes, which would be costly to recover from. 
To do this, they could leverage the features of the \sys{} system to ensure that their collaboration was organized and efficient, and that the data was protected from any unintended changes.
This scenario simulates the case where error recovery could be costly in a collaboration setting. 
}
\subsubsection{Scenario 3: Classroom Sharing with Hierarchical Permissions}
\add{In this scenario, we provided participants with an educational notebook on the topic of linear regression, taken from a data science handbook. 
The first half of the notebook demonstrated the concepts, while the second half contained an exercise for students to practice what they learned.
Participants were asked to plan the use of the notebook as an instructor, taking into account the needs of the entire class during a lecture. 
They needed to ensure that they could effectively explain the concepts to the students, while also providing them with an opportunity to practice individually on the exercise. 
Additionally, the exercise included a standard solution that the instructor may want to go over with the class after they have explored their own solutions. 
Participants were asked to plan how they would like to set up the collaborative notebook at the beginning of the lecture, and how they would modify the configurations as the lecture progressed.}
\begin{table}[]
    \centering
    {\add{
    \begin{tabular}{c p{5cm} c p{4cm}}
         \toprule
        \textbf{Session} & \textbf{Action or Strategy} & \textbf{Feature} & \textbf{PID}\\
         \midrule
         Paired & Nudge the clumsy collaborator to create parallel cells & Parallel Cell & P1-14\\
         Paired & Merge parallel cells & Parallel Cell & P1, P2, P3, P5, P9, P11, P12, P14\\
         \midrule
         Planning (1) & Lock cells for loading package and data & Cell-Level Access Control & P3, P7, P10, P12, P13, P14 \\
         Planning (1) & Lock future cells & Cell-Level Access Control & P6, P10 \\
         Planning (1) & Lock the original or a copied dataframe & Variable-Level Access Control & P3, P10, P12, P13, P14 \\
         Planning (1) & Create a copy of the dataframe & --  & P3, P7, P12 \\
         Planning (1) & Ask Bob to use parallel cells & Parallel Cell & P6, P9, P13\\
         \midrule
         Planning (2) & Lock cells for loading data & Cell-Level Access Control & P3, P6, P10, P12, P13, P14 \\
         Planning (2) & Change cells' edit access so that interns can not change each others’ code & Cell-Level Access Control & P9, P12 \\
         Planning (2) & Lock the shared dataframe & Variable-Level Access Control & P3, P6, P7, P10, P12, P13, P14 \\
         Planning (2) & Ask the interns to use the parallel cells 
         & Parallel Cell & P3, P6, P9\\
         Planning (2) & Create a copy of the dataframe if needed & -- & P7, P10 \\
         \midrule
         Planning (3) & Lock editing access for code cells in lecture notes & Cell-Level Access Control & P3, P6, P7, P9, P10, P12, P13, P14 \\
         Planning (3) & Lock reading access for code cells in lecture notes that are not covered yet & Cell-Level Access Control & P6, P10 \\
         Planning (3) & Lock reading access for the standard solution code cell in the exercise & Cell-Level Access Control &  P3, P6, P9, P10, P12, P14\\
         Planning (3) & Lock access for variables generated in lecture notes & Variable-Level Access Control & P13\\
         Planning (3) & Lock access for the variable for storing results in the exercise & Variable-Level Access Control & P14 \\
         Planning (3) & Create parallel cells for students to work on the exercise & Parallel Cell & P3, P7, P9, P10, P12, P13, P14 \\
         Planning (3) & Ask students to use parallel cells if they want to explore the code (e.g., change parameters) in lecture notes & Parallel Cell & P9, P12 \\
         \midrule
         Group & Create parallel cells & Parallel Cell & P3, P4, P7, P9, P10, P14 \\
         Group & Merge parallel cells & Parallel Cell & P4, P7, P9 \\
         Group & Sync parallel cells & Parallel Cell & P3 \\
         \bottomrule
    \end{tabular}
    }}
    \caption{\add{Features that participants have used for tasks in each study.}}
    \label{tab:strategy}
\end{table}

\add{\subsection{Data Analysis}}
\add{In each of the above scenarios, participants were asked to configure a shared notebook.
We used three metrics to understand and evaluate the effectiveness of the participants' specified notebook configurations.
% We collected three data sources to understand the effectiveness of the configuration. 
First, we summarize the patterns in how participants set up collaborative notebooks for each scenario. 
% Second, we identified and form lists of potential editing conflicts that might occur in each scenario.
The second data source was a list of potential editing conflicts that may occur in each scenario, which was identified by the research team. 
We used this list to test participants' configurations against the potential conflicts and analyze their reliability in addressing them. 
Lastly, we recorded and transcribed participants' post-task reflections, in which they discussed their choices, potential problems, and suggestions for additional features. 
These data sources gave us a comprehensive view of the effectiveness of the configuration in different collaboration scenarios.}
\add{\subsection{Results}}
\subsubsection{Usage of the Collaborative Features for Each Scenario}
\add{
In Table \ref{tab:strategy}, we summarize the strategies that participants described for each scenario and listed the features of \sys{} that are involved.
For the first scenario of working in an asynchronous paired programming session, three participants chose to ask the collaborator to use the parallel cells for exploration, while the other participants chose to use cell-level or variable-level access controls.
P12 explained why their strategy changed compared to the clumsy collaborator scenario in the previous paired session:
\begin{quote}
    I can't really trust that Bob is going to use parallel cells because we are not working together at the same time. I want to set up everything for him so he can only access the things he need.
\end{quote}}

\add{For the second scenario, most participants except P10 chose to lock the shared variable to prevent it from being polluted. 
Participants suggested that the interns could use parallel cells or make a copy of the dataframe if needed.
In addition, most participants (6 out of 8) chose to restrict the editing access of the code cell for loading the data, while two of them also chose to set up the editing access for the code cells that are assigned to each individual intern.}

\add{In the last scenario, participants described a mixed strategy for planning the collaborative notebook for a data science classroom.
All participants decided to turn off the editing access for code cells in lecture notes, as P14 explained:
\begin{quote}
    I would turn off the cell editing for the class. Otherwise, if there's so many students, it is easy for someone to accidentally hit a backspace somewhere or something and mess things up.
\end{quote}
Some participants (P9 and P12) mentioned that they would create a copy of the cell below each code cell for lecture notes and make them into parallel cells, in case students want to explore the code cells in lecture notes.
For the same consideration, P13 wanted to restrict the access for variables generated in lecture notes, in case students modify the shared runtime in lecture.
Other participants did not worry about protecting the shared variables, as one participant explained (P6):
\begin{quote}
    Since the content of the code cell is locked, I can always restart the kernel and run the notebook from the beginning if anything goes wrong.
\end{quote}
In addition, two participants (P6 and P10) mentioned that they would like to change the code cells' reading access as the lecture progresses so that students can stay focused.
For the exercise part, most participants planned to hide the reference solution code (6 out of 8) and ask students to work on parallel cells for their own practice (7 out of 8).}

\begin{table}[]
    \centering
    {\add{
    \begin{tabular}{c p{10cm} c c}
        \toprule
        \textbf{Scenario} & \textbf{Editing Conflicts} & \textbf{Category} & \textbf{Pass Rate}  \\
        \midrule
        Scenario 1 & Bob dropped all the NA values in the dataset. & Common & 0.75 \\
        Scenario 1 & Bob changed the importing package cell to only include a subset of a package. & Common & 0.75 \\
        Scenario 1 & Bob missed the instruction and started to work on the last code cell. & Rare & 0.25 \\
        \midrule
        Scenario 2 & Intern A changed the shared dataframe. & Common & 0.88 \\
        Scenario 2 & Intern A run the code cell for loading the data frame. & Common & 0.88 \\
        Scenario 2 & Intern A and intern B have the same naming of a variable. & Rare & 0.38 \\
        \midrule
        Scenario 3 & A student edited the code cells for demonstration. & Common & 1 \\
        Scenario 3 & Students directly assigned the prediction results to the shared data frame. & Common & 0.88 \\
        Scenario 3 & Students executed a code cell multiple times. & Rare & 0.13 \\
        \bottomrule
    \end{tabular}
    }}
    \caption{\add{For each scenario, the research team solicited three potential cases for editing conflicts and run through participants' notebooks through these cases.}}
    \label{tab:rubric}
\end{table}
\subsubsection{Effectiveness of the Collaboration Plan}
\add{For each scenario, we solicited three potential conflicts that may arise during collaboration: two that we expect to be common and one that is less likely to occur. 
We then evaluated each participant's use of the collaborative notebook to determine if their configuration could effectively address these conflicts. 
Two members of the research team carefully calibrated and discussed the ratings until they reached a consensus. 
The results, shown in Table \ref{tab:rubric}, indicate that most participants (more than 6 out of 8) were able to utilize the features in \sys{} to successfully address common collaboration issues. 
Even for the less likely problems (e.g., Bob missing the instruction and starting work on the last code cell in the first scenario), a small number of participants (1--3) were still able to successfully handle these rare cases.}
\subsubsection{Improving Access Control}
\add{In the reflective interview, participants mentioned several potential problems and suggested improvements for the collaboration scenarios in the current system design.}

\add{First, participants brought up the need for better access control on the notebook level. For example, P13 mentioned that restarting or interrupting the notebook kernel in the third collaboration scenario could cause problems when the instructor is demonstrating concepts. Other types of access control mentioned by participants included preventing collaborators from executing a code cell (P6) or copying and pasting the content from a code cell (P13).}

\add{Participants also suggested ways to improve the process of configuring access control. 
For example, in the first scenario, P6 and P10 mentioned that they would like to restrict cell edit access for their collaborator for every new code cell that they create under a section.
One participant also suggested adding a ``run and lock all cells and variables above'' button (P13) to avoid the need to manually lock all code cells in the lecture notes in the third scenario.}

\add{Lastly, participants (P9 and P12) mentioned the potential benefits of combining cell access control with parallel cells. This would be particularly useful in the third scenario, where the instructor may not want students to see each other's solutions in the parallel cell.}
